# Supplementary material for: Theory of Impedance Spectroscopy for Lithium Batteries
Source: arXiv:1908.00962 ancillary file (2019-08-02)
Supplement: Supplementary file 1 [file supporting_information.pdf]

# Electronic Supporting Information: Theory of Impedance Spectroscopy for Lithium Batteries

Fabian Single

*German Aerospace Center (DLR), Institute of Engineering Thermodynamics, Pfaffenwaldring 38-40, 70569 Stuttgart, Germany and Helmholtz Institute Ulm (HIU), Helmholtzstraße 11, 89081 Ulm, Germany*

Birger Horstmann* and Arnulf Latz†

*German Aerospace Center (DLR), Institute of Engineering Thermodynamics, Pfaffenwaldring 38-40, 70569 Stuttgart, Germany*

*Helmholtz Institute Ulm (HIU), Helmholtzstraße 11, 89081 Ulm, Germany and Ulm University, Albert-Einstein-Allee 47, 89081 Ulm, Germany*

(Dated: August 2, 2019)

## CONTENTS

SI-1. Transport Theory 2
A. Reference Velocity 3
B. Incompressibility and Convection 4
C. Thermodynamically consistent Flux Expressions 5

SI-2. Linearisation 9

SI-3. Binary Electrolyte 14
A. Chemical Potentials 16
B. Salt Diffusion Coefficient 18
C. Flux Expressions 19
D. Linearisation 20

SI-4. Impedance: Electroneutral System With SEI 21

SI-5. Appendix: General Impedance 21
A. Dispersion Relation 21
B. Double-Layer Thickness and Interface Capacity 23
C. Non-Neutral System without SEI 26
D. Non-Neutral System with SEI 27

SI-6. Intercalation Electrodes 29

SI-7. List of Parameters 32

References 33

## SI-1. TRANSPORT THEORY

The transport theory presented in this section is based on a publication by Schammer et al.[1] As mentioned in the main document, similar theories have been discussed in Refs.[2–4] The theory describes a liquid mixture of $N$ different species which are labelled with the subscript $\alpha = 1, \dots, N$. The special case of the binary electrolyte is discussed in section SI-3.

## A. Reference Velocity

The transport theory is derived relative to the center-of-mass velocity of the liquid. In contrast, the lab or resting frame is a global reference system which describes the mixture from an external perspective. Below, any quantity or parameter that is directly associated with the lab frame is marked with superscript $*$. Quantities and parameters without this label refer to the formulation relative to the center-of-mass velocity. Molar flux densities in both formulations are related

$$\mathrm{N}_\alpha^* = c_\alpha \mathrm{v}_\alpha^*, \tag{SI-1a}$$

$$\mathrm{N}_\alpha = c_\alpha \left(\mathrm{v}_\alpha^* - \mathrm{v}\right). \tag{SI-1b}$$

Here, $\mathrm{v}_\alpha^*$ is the mean velocity of species $\alpha$ in the lab frame. v is the center-of-mass velocity which is given by

$$\mathrm{v} = \frac{1}{\rho}\sum_{\alpha=1}^{N} \rho_\alpha \mathrm{v}_\alpha^*, \tag{SI-2}$$

where $\rho$ and $\rho_\alpha$ are the density of the mixture and the partial density of species $\alpha$. Any choice of reference system reduces the amount of independent fluxes by one. All individual fluxes relative to the center-of-mass velocity satisfy

$$0 = \sum_{\alpha=1}^{N} M_\alpha \mathrm{N}_\alpha, \tag{SI-3}$$

where $M_\alpha$ is the molar mass of species $\alpha$. In the derivation below, species 1 is chosen to be "eliminated" with this constraint. This suggests the definition of the following effective quantities which appear frequently below

$$\tilde{z}_\alpha = z_\alpha - \frac{M_\alpha}{M_1} z_1, \tag{SI-4a}$$

$$\tilde{\mu}_\alpha = \mu_\alpha - \frac{M_\alpha}{M_1} \mu_1, \tag{SI-4b}$$

$$\tilde{\nu}_\alpha = \nu_\alpha - \frac{M_\alpha}{M_1} \nu_1, \tag{SI-4c}$$

where $\alpha \neq 1$. Here, $\tilde{z}_\alpha$ is the effective charge number, $\tilde{\mu}_\alpha$ is the effective chemical potential, and $\tilde{\nu}_\alpha$ is the effective partial molar volume of species $\alpha$.

### B. Incompressibility and Convection

Liquids in general feature large bulk moduli in the GPa range. To put this into perspective, to obtain a relative volume change of 1 % of a material featuring a bulk modulus of 1 GPa requires a pressure change of approximately 100 atmospheres. The pressure differences in liquid battery systems are not nearly as large and any expansion or compression of the liquids described here can be safely neglected. However, one must consider that the liquid actually fills its given volume at any time. This is ensured by the following constraint

$$\sum_{\alpha=1}^{N} \nu_\alpha c_\alpha = 1, \tag{SI-5}$$

where $\nu_\alpha$ is the partial molar volume of species $\alpha$. It is defined by the volume change the system experiences if the number of particles of species $\alpha$ changes, $\nu_\alpha = \frac{\partial V}{\partial N_\alpha}$. The time derivative of this expression yields $\sum_\alpha (\dot{\nu}_\alpha c_\alpha + \nu_\alpha \dot{c}_\alpha) = 0$. Inserting the mass balance equations for $\dot{c}_\alpha$, see eq. (6), then results in an equation for the convective velocity

$$\begin{aligned} \nabla \mathrm{v} &= -\sum_{\alpha=1}^{N} \nu_\alpha \left( \nabla \mathrm{N}_\alpha - s_\alpha \right) \\ &= -\sum_{\alpha=2}^{N} \tilde{\nu}_\alpha \nabla \mathrm{N}_\alpha + \sum_{\alpha=1}^{N} \nu_\alpha s_\alpha, \end{aligned} \tag{SI-6}$$

In the second step we use eq. (SI-3) to eliminate the flux density of species 1. This is achieved with the effective partial molar volumes defined in eq. (SI-4c). Equation (SI-6) couples the net "volume" evolution to a change in the convection velocity. We integrate this equation to obtain an expression for center-of-mass velocity

$$\mathrm{v}(x) = \mathrm{v}(x_\mathrm{I}) + \int_{x_\mathrm{I}}^{x} \nabla \mathrm{v}(\tilde{x}) d\tilde{x}. \tag{SI-7}$$

Here, $x_\mathrm{I}$ is the location of an interface. Source are neglected because we only consider interface reactions only. Heterogeneous reactions are not considered in this work. Note that

the integral representation of v is only possible in a one dimensional system. This is not possible in higher dimensional systems where v is not rotation free.

Next, $\mathrm{v}(x_\mathrm{I})$ is calculated to obtain the flux boundary condition in the lab frame. Below, interface reactions will be considered which represent processes such as intercalation and deintercalation or metal deposition and stripping. The rate of these interface reactions is given by $j_\mathrm{I}$ in units of $\mathrm{A\,m^{-2}}$. It is now assumed that only one species labelled + can react at the interface. All other species $\alpha \neq +$ are inert and do not participate in the interface reaction. This implies

$$\mathrm{N}^*_+ = j^*_\mathrm{I}/z_+F, \tag{SI-8a}$$

$$\mathrm{N}^*_{\alpha\neq+} = 0, \tag{SI-8b}$$

where $\mathrm{N}^*_\alpha$ are the molar fluxes in the lab frame. Here, $j^*_\mathrm{I}$ is the sign adjusted interface flux which considers the orientation of the interface as well as the sign convention used for the interface reaction. Considering that $\mathrm{N}^*_\alpha = c_\alpha \mathrm{v}^*_\alpha$ as well as the definition for the center-of-mass velocity results in

$$\mathrm{v}\left(x_\mathrm{I}\right) = \frac{1}{\rho}\sum_{\alpha=1}^{N}\rho_\alpha \mathrm{v}^*_\alpha\left(x_\mathrm{I}\right) = \frac{\rho_+}{\rho}\mathrm{v}^*_+ = \frac{1}{c_+}\frac{\rho_+}{\rho}\frac{j^*_\mathrm{I}}{z_+F} \tag{SI-9}$$

Inserting this expression in eq. (SI-8) results in the final set of boundary conditions

$$\mathrm{N}^*_\alpha\left(x_\mathrm{I}\right) = \mathrm{N}_\alpha + c_\alpha \mathrm{v} = \mathrm{N}_\alpha + \frac{c_\alpha}{c_+}\frac{\rho_+}{\rho}\frac{j^*_\mathrm{I}}{z_+F} = \begin{cases} \frac{j^*_\mathrm{I}}{z_+F} & \alpha = +, \\ 0 & \text{otherwise.} \end{cases} \tag{SI-10}$$

It is evident that the choice of the center-of-mass reference is reflected in this expression as the additional term obtained by considering convection is proportional to the mass ratio $\rho_+/\rho$.

### C. Thermodynamically consistent Flux Expressions

The Onsager Ansatz relates all general forces within the system $\nabla\tilde{\mu}^\mathrm{el}_\alpha = \nabla\tilde{\mu}_\alpha + F\tilde{z}_\alpha\nabla\phi_\mathrm{E}$ to the $N-1$ independent particle fluxes $\mathrm{N}_\alpha$. It guarantees that entropy production is positive

which means that the theory below satisfies the second law of thermodynamics, see Ref.[1]

$$\begin{pmatrix} \mathrm{N}_2 \\ \vdots \\ \mathrm{N}_N \end{pmatrix} = -\begin{pmatrix} \Gamma_{22} & \dots & \Gamma_{2N} \\ \vdots & \ddots & \\ \Gamma_{N2} & & \Gamma_{NN} \end{pmatrix} \begin{pmatrix} \nabla\tilde{\mu}_2^{\mathrm{el}} \\ \vdots \\ \nabla\tilde{\mu}_N^{\mathrm{el}} \end{pmatrix}. \tag{SI-11}$$

Below, the Onsager matrix $\boldsymbol{\Gamma}$ and its coefficients $\Gamma_{\alpha\beta}$ are also referred to as mobility matrix and mobility coefficients. Note that these fluxes are relative to the center-of-mass velocity. Therefore, only $N-1$ individual fluxes exist and $\mathrm{N}_1$ can be obtained from eq. (SI-3). The mobility matrix comprises all transport processes and its entries determine the corresponding transport parameters. Considering its symmetry, $(N-1)(N-2)/2$ transport parameters need to be defined. Inserting $\nabla\tilde{\mu}_\alpha^{\mathrm{el}}$ and stating each flux expressions individually leads to

$$\mathrm{N}_\alpha = -\sum_{\beta=2}^{N} \Gamma_{\alpha\beta}\nabla\tilde{\mu}_\beta - F\sum_{\beta=2}^{N} \tilde{z}_\beta\Gamma_{\alpha\beta}\nabla\phi_{\mathrm{E}}, \text{ and} \tag{SI-12a}$$

$$\mathcal{J} = -F\sum_{\alpha,\beta=2}^{N} \tilde{z}_\alpha\Gamma_{\alpha\beta}\nabla\tilde{\mu}_\alpha - F^2\sum_{\alpha,\beta=2}^{N} \tilde{z}_\alpha\tilde{z}_\beta\Gamma_{\alpha\beta}\nabla\phi_{\mathrm{E}}. \tag{SI-12b}$$

The expression for the charge flux relative to the center-of-mass velocity is obtained by summing all $N-1$ independent fluxes weighted with the effective charge numbers $\tilde{z}_\alpha$, see eq. (SI-4a). By comparison with the canonical form of the electric current in ionic systems we can then identify transport parameters commonly used in literature such as the conductivity $\kappa$ as well as the transference numbers $t_\alpha$ ($\alpha \geq 2$)

$$\kappa = F^2\sum_{\alpha,\beta=2}^{N} \tilde{z}_\alpha\tilde{z}_\beta\boldsymbol{\Gamma}_{\alpha\beta}, \tag{SI-13a}$$

$$t_\alpha = \frac{F^2}{\kappa}\sum_{\beta=2}^{N} \tilde{z}_\alpha\tilde{z}_\beta\boldsymbol{\Gamma}_{\alpha\beta}. \tag{SI-13b}$$

There are $N-2$ independent transference numbers as $\sum_{\alpha=2}^{N} t_\alpha = 1$. These transference numbers describe fluxes relative to the center-of-mass velocity, they are not applicable in different reference systems. They also depend on the specific choice of species "1" because this choice affects the effective charge numbers $\tilde{z}_\alpha$. With these expressions the equations

above become

$$\mathrm{N}_\alpha = -\sum_{\beta=2}^{N} \mathbf{\Gamma}_{\alpha\beta} \nabla \tilde{\mu}_\beta - \frac{t_\alpha \kappa}{\tilde{z}_\alpha F} \nabla \phi_{\mathrm{E}}, \tag{SI-14a}$$

$$\mathcal{J} = -\frac{\kappa}{F} \sum_{\alpha=2}^{N} \frac{t_\alpha}{\tilde{z}_\alpha} \nabla \tilde{\mu}_\alpha - \kappa \nabla \phi_{\mathrm{E}}. \tag{SI-14b}$$

Rearranging eq. (SI-14b) for the potential and eliminating the former in eq. (SI-14a) results in another, frequently used form of the flux expression

$$\mathrm{N}_\alpha = -\sum_{\beta=2}^{N} \left( \mathbf{\Gamma}_{\alpha\beta} - \frac{t_\alpha t_\beta \kappa}{z_\alpha z_\beta F^2} \right) \nabla \tilde{\mu}_\beta + \frac{t_\alpha \mathcal{J}}{z_\alpha F}, \tag{SI-15}$$

which motivates the introduction of the shifted mobility matrix $\tilde{\mathbf{\Gamma}}$ with the coefficients

$$\tilde{\Gamma}_{\alpha\beta} = \Gamma_{\alpha\beta} - \frac{t_\alpha t_\beta \kappa}{z_\alpha z_\beta F^2}. \tag{SI-16}$$

The shifted mobility coefficients $\Gamma_{\alpha\beta}$ are not independent which becomes obvious when calculating their weighted sum

$$\sum_{\beta=2}^{N} \tilde{z}_\beta \tilde{\mathbf{\Gamma}}_{\alpha\beta} = 0 \qquad \Longrightarrow \qquad \tilde{\mathbf{\Gamma}}_{\alpha 2} = -\frac{1}{\tilde{z}_2} \sum_{\beta=3}^{N} \tilde{z}_\beta \tilde{\mathbf{\Gamma}}_{\alpha\beta}. \tag{SI-17}$$

This can be used to simplify the flux expression eq. (SI-15) for all species $\alpha \geq 3$

$$\begin{aligned} \mathrm{N}_\alpha &= -\sum_{\beta=3}^{N} \tilde{\mathbf{\Gamma}}_{\alpha\beta} \nabla \left( \tilde{\mu}_\beta - \frac{\tilde{z}_\beta}{\tilde{z}_2} \tilde{\mu}_2 \right) + \frac{t_\alpha \mathcal{J}}{\tilde{z}_\alpha F} \\ &= -\sum_{\beta=3}^{N} \tilde{\mathbf{\Gamma}}_{\alpha\beta} \nabla \tilde{\tilde{\mu}}_\alpha + \frac{t_\alpha \mathcal{J}}{\tilde{z}_\alpha F}. \end{aligned} \tag{SI-18}$$

Here, the "effective" effective chemical potential of the salt has been introduced as

$$\tilde{\tilde{\mu}}_\alpha = \tilde{\mu}_\alpha - \frac{\tilde{z}_\alpha}{\tilde{z}_2} \tilde{\mu}_2. \tag{SI-19}$$

Now, the electric current, see eq. (SI-14b), is expressed with these quantities. Directly

exchanging $\tilde{\mu}_\alpha$ with $\tilde{\tilde{\mu}}_\alpha$ and running the sum from 3 instead of 2 results in

$$\begin{aligned}\sum_{\alpha=3}^{N} \frac{t_\alpha}{\tilde{z}_\alpha} \nabla \tilde{\tilde{\mu}}_\alpha &= \sum_{\alpha=3}^{N} \frac{t_\alpha}{\tilde{z}_\alpha} \nabla \tilde{\mu}_\alpha - \sum_{\alpha=3}^{N} \frac{t_\alpha}{\tilde{z}_2} \nabla \tilde{\mu}_2 \\ &= \sum_{\alpha=3}^{N} \frac{t_\alpha}{\tilde{z}_\alpha} \nabla \tilde{\mu}_\alpha - \frac{1-t_2}{\tilde{z}_2} \nabla \tilde{\mu}_2 \\ &= \sum_{\alpha=2}^{N} \frac{t_\alpha}{\tilde{z}_\alpha} \nabla \tilde{\mu}_\alpha - \frac{\nabla \tilde{\mu}_2}{\tilde{z}_2}. \end{aligned} \tag{SI-20}$$

This substitution results in an extra term which is now absorbed in the electrochemical potential defined as

$$\tilde{\varphi} = \phi_{\mathrm{E}} + \frac{\tilde{\mu}_2}{\tilde{z}_2 F}. \tag{SI-21}$$

Then, the final expression for the electric current reads

$$\mathcal{J} = -\frac{\kappa}{F} \sum_{\alpha=3}^{N} \frac{t_\alpha}{\tilde{z}_\alpha} \nabla \tilde{\tilde{\mu}}_\alpha - \kappa \nabla \tilde{\varphi}. \tag{SI-22}$$

To conclude, to describe the temporal evolution of a mixture of $N$ species, $N-1$ mass balance equations need to be solved, see eq. (6). These mass balance equations can be written for an arbitrary subset of concentrations $c_\alpha$ and the charge density $\varrho$. There are only $N-1$ independent fluxes relative to the center-of-mass velocity. They are driven by $N-2$ effective effective chemical potentials $\tilde{\tilde{\mu}}_\alpha$ and the electrochemical potential $\tilde{\varphi}$. To transform these fluxes into the resting frame, one additional equation (constraint) needs to be considered to find the convective velocity. We assume incompressibility and determine the convection velocity by eq. (SI-6). In non-neutral systems the Poisson equation can be used to relate the potential to the concentration distribution. This is not necessary in neutral systems where the assumption of electroneutrality implies $\varrho = 0$, reducing the number of independent concentrations by one. Then, the potential can be calculated with eq. (SI-22) or eq. (SI-14b).

Most flux expressions derived above will be used in mass-balance equations where concentrations are used as primary variables. It is therefore desirable to express all fluxes with concentration gradients instead of chemical potential gradients. Expanding the following

expression

$$\sum_{\beta=2}^{N} \Gamma_{\alpha\beta} \nabla \tilde{\mu}_\beta = \sum_{\beta=2}^{N} \sum_{\gamma=2}^{N} \Gamma_{\alpha\beta} \frac{\partial \tilde{\mu}_\beta}{\partial c_\gamma} \nabla c_\gamma$$

yields

$$D_{\alpha\beta} = \sum_{\gamma=2}^{N} \Gamma_{\alpha\gamma} \frac{\partial \tilde{\mu}_\gamma}{\partial c_\beta}, \qquad \boldsymbol{D} = \boldsymbol{\Gamma} \boldsymbol{J}_{\tilde{\mu}}, \tag{SI-23a}$$

$$\tilde{D}_{\alpha\beta} = \sum_{\gamma=2}^{N} \tilde{\Gamma}_{\alpha\gamma} \frac{\partial \tilde{\mu}_\gamma}{\partial c_\beta}. \qquad \tilde{\boldsymbol{D}} = \tilde{\boldsymbol{\Gamma}} \boldsymbol{J}_{\tilde{\mu}}, \tag{SI-23b}$$

Here, the diffusion matrix is expressed element wise in sum notation on the left and in matrix notation on the right. $\boldsymbol{J}_{\tilde{\mu}}$ is the Jacobi matrix of $\tilde{\mu}_\alpha$ with respect to $c_\alpha$ ($\alpha = 2, \ldots, N$). With this, the particle flux expressions become

$$\mathrm{N}_\alpha = -\sum_{\beta=2}^{N} D_{\alpha\beta} \nabla c_\alpha - \frac{t_\alpha \kappa}{z_\alpha F} \nabla \phi_{\mathrm{E}}, \tag{SI-24a}$$

$$\mathrm{N}_\alpha = -\sum_{\beta=2}^{N} \tilde{D}_{\alpha\beta} \nabla c_\alpha + \frac{t_\alpha \mathcal{J}}{z_\alpha F}, \tag{SI-24b}$$

for all $\alpha \geq 2$. Both $\boldsymbol{D}$ and $\tilde{\boldsymbol{D}}$ are $N-1 \times N-1$ matrices. In addition, the effective shifted diffusion matrix is introduced which is a $N-2 \times N-2$ matrix because $\tilde{\tilde{\mu}}_\alpha$ is only defined for $\alpha \geq 3$

$$\tilde{\tilde{D}}_{\alpha\beta} = \sum_{\gamma=3}^{N} \Gamma_{\alpha\gamma} \frac{\partial \tilde{\tilde{\mu}}_\gamma}{\partial c_\beta}. \qquad \tilde{\tilde{\boldsymbol{D}}} = \tilde{\boldsymbol{\Gamma}} \boldsymbol{J}_{\tilde{\tilde{\mu}}}. \tag{SI-25}$$

## SI-2. LINEARISATION

Any perturbation applied to the system is small and the deviation from the equilibrium state is denoted as

$$\delta c_\alpha(x,t) = c_\alpha(t,x) - c_{\alpha,0}, \tag{SI-26a}$$

$$\delta \phi_{\mathrm{E}}(t,x) = \phi_{\mathrm{E}}(t,x) - \phi_{\mathrm{E},0}. \tag{SI-26b}$$

Here, the reference concentration and potential in the electrolyte are constant in space and time. Next, we linearise the flux expression relative to the center-of-mass velocity. To this aim the perturbation variables are inserted into the flux expression given by eq. (SI-24a). Then all parameters with a concentration dependence ($D_{\alpha\beta}$, $t_\alpha$, and $\kappa$) are approximated with a first order series expansion in $c_\alpha$

$$\begin{aligned}
\mathrm{N}_\alpha &= -\sum_{\beta=2}^{N} D_{\alpha\beta} \nabla c_\beta + \frac{t_\alpha \kappa}{z_\alpha F} \nabla \phi_\mathrm{E} \\
&= -\sum_{\beta=2}^{N} D_{\alpha\beta} \nabla \delta c_\beta + \frac{t_\alpha \kappa}{z_\alpha F} \nabla \delta \phi_\mathrm{E} \\
&= -\sum_{\beta=2}^{N} D_{\alpha\beta,\mathrm{lin}} \nabla \delta c_\beta + \frac{t_{\alpha,\mathrm{lin}} \kappa_\mathrm{lin}}{z_\alpha F} \nabla \delta \phi_\mathrm{E} + \mathcal{O}\left(\delta^2\right). \qquad \text{(SI-27)}
\end{aligned}$$

Here, $\delta^2$ comprises all quadratic combinations of perturbation variables ($\delta c_1$, $\delta c_1 \delta c_2$, $\delta c_2^2$, etc.) and the first order approximation of the quantity $\xi$ is given by

$$\xi_\mathrm{lin} = \underbrace{\xi\left(c_{1,0}, \ldots, c_{N,0}\right)}_{\xi_0} + \sum_{\beta=1}^{N} \left.\frac{\partial \xi}{\partial c_\beta}\right|_{c_\alpha = c_{\alpha,0}} \cdot \delta c_\beta + \mathcal{O}\left(\delta^2\right). \qquad \text{(SI-28)}$$

In the first order approximation of eq. (SI-27) all terms of higher order in the deviation variables can be omitted. Only first order terms in perturbation variables remain

$$\mathrm{N}_{\alpha,\mathrm{lin}} = -\sum_{\beta=2}^{N} D_{\alpha\beta,0} \nabla \delta c_\beta + \frac{t_{\alpha,0} \kappa_0}{z_\alpha F} \nabla \delta \phi_\mathrm{E}. \qquad \text{(SI-29)}$$

It can be seen that concentration dependence of the transport parameters disappears in the linearised flux expression. Furthermore, all former variables are now replaced with their corresponding perturbation variable. The linearised flux expression consists of first order terms in deviation variables only. Naturally, there is no zero order term because the reference state is in equilibrium. Next, the expression for the convection velocity (derived from the

assumption of incompressibility see eq. (SI-6)) is linearised as well

$$\begin{aligned}\nabla \mathrm{v} &= -\sum_{\alpha=2}^{N} \tilde{\nu}_\alpha \nabla \mathrm{N}_\alpha \\ &= -\sum_{\alpha=2}^{N} \tilde{\nu}_{\alpha,\mathrm{lin}} \nabla \mathrm{N}_{\alpha,\mathrm{lin}} + \mathcal{O}\left(\delta^2\right) \\ \Longrightarrow \left(\nabla \mathrm{v}\right)_{\mathrm{lin}} &= -\sum_{\alpha=2}^{N} \tilde{\nu}_{\alpha,0} \nabla \mathrm{N}_{\alpha,\mathrm{lin}}. \end{aligned} \tag{SI-30}$$

Note that the production term $s$ is omitted because only interface reactions are considered. The concentration dependence of $\tilde{\nu}_\alpha$ is omitted because $\mathrm{N}_{\alpha,\mathrm{lin}}$ has no zero-order terms as ascertained above (flux free reference state). Integration then yields the first order approximation of the convection velocity

$$\begin{aligned}\mathrm{v}_{\mathrm{lin}} &= -\sum_{\alpha=2}^{N} \tilde{\nu}_{\alpha,0} \left(\mathrm{N}_{\alpha,\mathrm{lin}} - \mathrm{N}_{\alpha,\mathrm{lin}}\left(x_{\mathrm{I}}\right)\right) + \mathrm{v}\left(x_{\mathrm{I}}\right), \\ &= -\sum_{\alpha=2}^{N} \tilde{\nu}_{\alpha,0} \mathrm{N}_{\alpha,\mathrm{lin}} + \mathrm{v}_{\mathrm{off}} \end{aligned} \tag{SI-31}$$

where $x_{\mathrm{I}}$ is the location of an interface and $\mathrm{v}\left(x_{\mathrm{I}}\right)$ is the center-of-mass velocity caused by reactions (particle sources) at the interface. The offset velocity $\mathrm{v}_{\mathrm{off}} = \sum_{\alpha=2}^{N} \tilde{\nu}_{\alpha,0} \mathrm{N}_{\alpha,\mathrm{lin}}\left(x_{\mathrm{I}}\right) + \mathrm{v}\left(x_{\mathrm{I}}\right)$ comprises all terms in the flux expression that can be attributed to the interface reaction. These contributions are constant in space such that $\nabla \cdot \mathrm{v}_{\mathrm{off}} = 0$. Using the linearised expression for v and $\mathrm{N}_\alpha$ the linearised fluxes in the resting frame become

$$\begin{aligned}\mathrm{N}^*_{\alpha,\mathrm{lin}} &= \mathrm{N}_{\alpha,\mathrm{lin}} + c_{\alpha,0} \mathrm{v}_{\mathrm{lin}} \\ &= \sum_{\beta=2}^{N} \left(\delta_{\alpha\beta} - c_{\alpha,0} \tilde{\nu}_{\beta,0}\right) \mathrm{N}_{\beta,\mathrm{lin}} + c_{\alpha,0} \mathrm{v}_{\mathrm{off}}, \end{aligned} \tag{SI-32}$$

where $\delta_{\alpha\beta}$ is the Kronecker delta. This linear relation between the fluxes relative to the center-of-mass velocity and the fluxes in the resting frame can be written in matrix form.

To this aim, we condense concentrations and fluxes into vectors

$$\begin{pmatrix} \mathrm{N}^*_{2,\mathrm{lin}} \\ \vdots \\ \mathrm{N}^*_{N,\mathrm{lin}} \end{pmatrix} = \underbrace{\left[ \boldsymbol{\mathcal{I}} - \begin{pmatrix} c_{2,0}\tilde{\nu}_{2,0} & \dots & c_{2,0}\tilde{\nu}_{N,0} \\ \vdots & \ddots & \vdots \\ c_{N,0}\tilde{\nu}_{2,0} & \dots & c_{N,0}\tilde{\nu}_{N,0} \end{pmatrix} \right]}_{\boldsymbol{\mathcal{C}}} \begin{pmatrix} \mathrm{N}_{2,\mathrm{lin}} \\ \vdots \\ \mathrm{N}_{N,\mathrm{lin}} \end{pmatrix} + \vec{c}_0 \mathrm{v}_{\mathrm{off}}. \tag{SI-33}$$

Here, $\boldsymbol{\mathcal{I}}$ is the identity matrix. Vector quantities $\vec{\xi}$ contain the elements $\xi_2, \dots, \xi_N$ . Below, $\boldsymbol{\mathcal{C}}$ is referred to as the convection-correction matrix. It can be written as

$$\boldsymbol{\mathcal{C}} = \boldsymbol{\mathcal{I}} - \vec{c}_0 \vec{\tilde{\nu}}_0^T, \tag{SI-34}$$

where the $\vec{c}_0$ and $\vec{\tilde{\nu}}_0$ are vectors with the entries $c_{\alpha,0}$ and $\tilde{\nu}_{\alpha,0}$, $\alpha = 2, \dots, N$. We use Sylvester's determinant theorem to calculate the determinant of this matrix (first step)

$$\begin{aligned} \det \boldsymbol{\mathcal{C}} &= 1 - \vec{\tilde{\nu}}_0^T \vec{c}_0 = 1 - \sum_{\alpha=2}^{N} c_{\alpha,0}\tilde{\nu}_{\alpha,0} \\ &= 1 - \sum_{\alpha=2}^{N} c_{\alpha,0} \left( \nu_{\alpha,0} - \frac{M_\alpha}{M_1}\nu_{1,0} \right) \\ &= \frac{1}{M_1} \left[ M_1 c_{1,0}\nu_{1,0} + \sum_{\alpha=2}^{N} M_\alpha c_{\alpha,0}\nu_{1,0} \right] \\ &= \frac{\nu_{1,0}}{M_1}\rho_0 = \frac{\rho_0}{\tilde{\rho}_{1,0}}. \end{aligned} \tag{SI-35}$$

We use the definition of $\tilde{\nu}_\alpha$ in the second line and $\rho = \sum_{\alpha=1}^{N} M_\alpha c_\alpha$ in the third line. It can be seen that the determinant can be reduced to the ratio of two densities. This means that the determinant is nonzero and that $\boldsymbol{\mathcal{C}}$ can be inverted. Here $\rho_0$ is the mass density of the mixture in the reference state. In contrast, $\tilde{\rho}_{1,0}$ is the extrapolated density of species 1. This quantity must be calculated from the partial molar volume of this species in the reference state $\tilde{\rho}_{1,0} = \frac{M_1}{\nu_{1,0}}$.

Using the the matrix form of the fluxes relative to the center-of-mass velocity and trans-

forming them into the resting frame with eq. (SI-33) results in

$$\begin{aligned}\vec{\mathrm{N}}^{*} &= \boldsymbol{\mathcal{C}}\boldsymbol{D}\nabla\vec{\delta c} + \boldsymbol{\mathcal{C}}\vec{T}\frac{\kappa}{F}\nabla\delta\phi_{\mathrm{E}} + \vec{c}_0\mathrm{v}_{\mathrm{off}},\\ &= \boldsymbol{D}^{*}\nabla\vec{\delta c} + \vec{T}^{*}\frac{\kappa}{F}\nabla\delta\phi_{\mathrm{E}} + \vec{c}_0\mathrm{v}_{\mathrm{off}},\end{aligned} \tag{SI-36}$$

where $\vec{T}_\alpha = \frac{t_\alpha}{\tilde{z}_\alpha}$ and $\vec{T^*}_\alpha = \frac{t^*_\alpha}{\tilde{z}_\alpha}$ $(\alpha = 2, \ldots, N)$. It can be seen that the flux expression in the resting frame has the exact same form as the one for fluxes relative to the center-of-mass velocity. These expressions only differ in the "offset flux" $\mathrm{v}_{\mathrm{off}}$ and the fact that a modified set of transport parameters are used. Note that only the entries of the diffusion matrix and the transference numbers need to be transformed whereas the conductivity remains the same in both frames

$$\boldsymbol{D}^{*} = \boldsymbol{\mathcal{C}}\boldsymbol{D}, \tag{SI-37a}$$

$$\vec{T}^{*} = \boldsymbol{\mathcal{C}}\vec{T}. \tag{SI-37b}$$

If all species $\alpha \geq 2$ have non zero $\tilde{z}_\alpha$, eq. (SI-37b) can be rewritten to relate the transference numbers in both frames directly

$$\vec{t^{*}} = \begin{pmatrix} \tilde{z}_2 & & 0 \\ & \ddots & \\ 0 & & \tilde{z}_{\mathrm{N}} \end{pmatrix} \boldsymbol{\mathcal{C}} \begin{pmatrix} \tilde{z}_2^{-1} & & 0 \\ & \ddots & \\ 0 & & \tilde{z}_{\mathrm{N}}^{-1} \end{pmatrix} \vec{t} \tag{SI-38}$$

These equations relate the transport parameters which describe fluxes relative to the center-of-mass velocity with the ones used in the resting frame flux expression. They can be inverted because $\boldsymbol{\mathcal{C}}$ has a non-zero determinant. Note that this set of resting frame transport parameters is a result of the first order approximation around a reference state which is in thermodynamic equilibrium. Therefore, these parameters can only be used in this very context. They can not be used to write down the fluxes in the resting frame if this condition is not met.

## SI-3. BINARY ELECTROLYTE

The binary electrolyte consists of a charge neutral solvent species (labelled N) as well as cations M and anions A (labelled + and −). Considering section SI-1, the former numeric labels are now assigned as $1 \to N$, $2 \to +$, and $3 \to -$. Cations and anions are added to the solution by adding a salt which is fully dissociated in the solvent

$$\mathrm{M}_{n_+}\mathrm{A}_{n_-} \longrightarrow n_+\mathrm{M}^{z_+} + n_-\mathrm{A}^{z_-}. \tag{SI-39}$$

The stoichiometric coefficients and the charge numbers satisfy

$$n_+ z_+ + n_- z_- = 0. \tag{SI-40}$$

With the framework derived in section SI-1 the solvent species is eliminated by describing the fluxes relative to the center-of-mass velocity. Also, because the solvent species is neutral, the effective charge numbers equal the original ones $\tilde{z}_\alpha = z_\alpha$, see eq. (SI-4a).

In the flux expressions derived in section SI-1, all transport parameters appear together with entries of the mobility matrix $\mathbf{\Gamma}$. However, the entries of the mobility matrix are directly related to the common, more accessible parameters with eqs. (SI-13a) and (SI-13b). In the case of a binary electrolyte, these equations read

$$\kappa = F^2 \left( z_+^2 \Gamma_{++} + 2 z_+ z_- \Gamma_{+-} + z_-^2 \Gamma_{--} \right), \tag{SI-41a}$$

$$t_+ \kappa = F^2 \left( z_+^2 \Gamma_{++} + z_+ z_- \Gamma_{+-} \right). \tag{SI-41b}$$

One goal of this section is to invert these relations to express the Onsager matrix $\mathbf{\Gamma}$ as a function of common transport parameters. To this aim, a third equation is needed to link the final common transport parameter to the mobility coefficients. The parameter in question is the salt diffusion coefficient $D_{\text{salt}}$. This parameter describes a collective diffusive motion of cations and anions on “large” scales. On these scales both ionic species cannot diffuse independently as this would cause charge separation. Therefore, salt diffusion is a charge-neutral process and electroneutrality is assumed to derive this final equation. This implies that the charge density $\varrho = F\left(z_+ c_+ + z_- c_-\right)$ is zero which directly relates both ionic

concentrations and their gradients, motivating the introduction of the salt concentration

$$c_{\text{salt}} = \frac{c_+}{n_+} = \frac{c_-}{n_-}. \tag{SI-42}$$

To find the missing equation, we need to express the gradient of the "effective-effective"-chemical potential $\tilde{\tilde{\mu}}_-$. With eq. (SI-40) as well as the definition of $\tilde{\tilde{\mu}}_-$, eq. (SI-19) it follows that

$$\tilde{\tilde{\mu}}_- = \tilde{\mu}_- - \frac{z_-}{z_+}\tilde{\mu}_+ = \tilde{\mu}_- + \frac{n_+}{n_-}\tilde{\mu}_+, \tag{SI-43}$$

which is true because $\tilde{z}_\alpha = z_\alpha$. This motivates the introduction of $\tilde{\mu}_{\text{salt}}$, the effective chemical potential of the salt

$$\begin{aligned}\tilde{\mu}_{\text{salt}} = \frac{n_-\tilde{\tilde{\mu}}_-}{n_+ + n_-} &= \frac{n_+\tilde{\mu}_+ + n_-\tilde{\mu}_-}{n_+ + n_-} \\ &= \underbrace{\frac{n_+\mu_+ + n_-\mu_-}{n_+ + n_-}}_{\mu_{\text{salt}}} - \frac{n_+M_+ + n_-M_-}{(n_+ + n_-)\,M_{\text{N}}}\mu_{\text{N}}.\end{aligned} \tag{SI-44}$$

Note that $\tilde{\mu}_{\text{salt}}$ contains weighted contributions from the solvent chemical potential. These originate from the description relative to the center-of-mass velocity. It must not be confused with $\mu_{\text{salt}}$ which only takes potential contributions of the ionic species into account. We use the Gibbs-Duhem relation to express the chemical potential of the solvent

$$\sum_{\alpha=\text{N},\pm} c_\alpha \text{d}\mu_\alpha = \frac{S}{V}\text{d}T + \text{d}P. \tag{SI-45}$$

Here, $S$ is entropy and $V$ is the volume of the system. $\text{d}T$ and $\text{d}P$ are temperature and pressure change which are zero because we assume constant temperature and pressure. This results in

$$\begin{aligned}c_{\text{N}}d\mu_{\text{N}} &= -\left(c_+d\mu_+ + c_-d\mu_-\right) = -c_{\text{salt}}\left(n_+d\mu_+ + n_-d\mu_-\right) \\ &= -c_{\text{salt}}\left(n_+ + n_-\right)d\mu_{\text{salt}}.\end{aligned} \tag{SI-46}$$

Considering this in the differential version of eq. (SI-44) gives

$$\frac{d\tilde{\mu}_{\text{salt}}}{dc_{\text{salt}}} = \frac{c_{\text{N}}M_{\text{N}} + c_+M_+ + c_-M_-}{c_{\text{N}}M_{\text{N}}}\frac{d\mu_{\text{salt}}}{dc_{\text{salt}}} = \frac{\rho}{\rho_{\text{N}}}\frac{d\mu_{\text{salt}}}{dc_{\text{salt}}}. \tag{SI-47}$$

The factor $\frac{\rho}{\rho_{\text{N}}}$ is larger than one and becomes one if the weight percentage of the salt is small, which corresponds to the dilute limit.

### A. Chemical Potentials

Generally, each chemical potential is a function of temperature, pressure, and the three concentrations $\mu_\alpha = \mu_\alpha(T, P, c_{\text{N}}, c_+, c_-)$. Both, temperature and pressure are assumed to be constant in this work. This leaves three concentrations, two of which are independent due to the volume constraint eq. (SI-5). Electroneutrality is another constraint in experiments because non-neutral solutions cannot be created. Therefore, one can only measure how the chemical potentials depend on the salt concentration. Electroneutrality is a good approximation within the bulk solution. However, the theory developed here also describes the electrolyte near interfaces where charged double-layers violate charge neutrality. For this reason, the following concentration dependence of the chemical potentials is assumed

$$\mu_\pm = RT\ln\left(\frac{f_\pm c_\pm}{c_{\pm,0}}\right). \tag{SI-48}$$

Here, $f_\alpha$ is the activity coefficient of the species $\alpha$ which depends on $c_\alpha$ only. The experimentally available activity coefficient of the salt mixture is linked to the activity coefficient of each ionic species

$$f_{\text{salt}}^{n_+ + n_-} = f_+^{n_+} f_-^{n_-}. \tag{SI-49}$$

This is consistent with the definition of $\mu_{\text{salt}}$ in eq. (SI-44). The thermodynamic factor of the salt is defined as $\mathcal{F}_{\text{salt}} = 1 + \frac{d\ln f_{\text{salt}}}{d\ln c_{\text{salt}}}$ and is linked to the thermodynamic factor of the individual ions. We use the definition of $\mu_{\text{salt}}$ and $f_{\text{salt}}$ in eqs. (SI-44) and (SI-49) which

results in

$$\mathcal{F}_{\text{salt}} = \frac{n_+ \mathcal{F}_+ + n_- \mathcal{F}_-}{n_+ + n_-}. \tag{SI-50}$$

Next, the dimensionless parameter $0 < \gamma < 1$ is introduced. It describes an asymmetry in the contribution of the individual ions to the thermodynamic factor of the salt

$$\mathcal{F}_+ = \gamma \cdot \frac{n_+ + n_-}{n_+} \mathcal{F}_{\text{salt}}, \tag{SI-51a}$$

$$\mathcal{F}_- = (1-\gamma) \cdot \frac{n_+ + n_-}{n_-} \mathcal{F}_{\text{salt}}. \tag{SI-51b}$$

Considering the definition of $c_{\text{salt}}$ and $\mu_\alpha$, see eqs. (SI-42) and (SI-48), as well of the simple concentration dependence of $f_\alpha$ then results in

$$\frac{\partial \mu_+}{\partial c_+} = \gamma \cdot \frac{n_+ + n_-}{n_+^2} \frac{d\mu_{\text{salt}}}{dc_{\text{salt}}}, \tag{SI-52a}$$

$$\frac{\partial \mu_-}{\partial c_-} = (1-\gamma) \cdot \frac{n_+ + n_-}{n_-^2} \frac{d\mu_{\text{salt}}}{dc_{\text{salt}}}. \tag{SI-52b}$$

Next, we calculate the Jacobi matrix of the effective potentials $\tilde{\mu}_\alpha$. This quantity is needed to find the diffusion matrix $\boldsymbol{D}$ which is used in eqs. (SI-24a) and (SI-24b). Again, the Gibbs-Duhem relation at constant temperature and pressure is used to express partial derivatives of $\mu_{\text{N}}$, see eq. (SI-46). We then obtain the Jacobi matrix of $\tilde{\mu}_\alpha$ with respect to $c_\alpha$

$$\boldsymbol{J}_{\tilde{\mu}} = \begin{pmatrix} \left(1 + \frac{\rho_+}{\rho_{\text{N}}}\right) \frac{\partial \mu_+}{\partial c_+} & \frac{M_+ c_-}{\rho_{\text{N}}} \frac{\partial \mu_-}{\partial c_-} \\ \frac{M_- c_+}{\rho_{\text{N}}} \frac{\partial \mu_+}{\partial c_+} & \left(1 + \frac{\rho_-}{\rho_{\text{N}}}\right) \frac{\partial \mu_-}{\partial c_-} \end{pmatrix}. \tag{SI-53}$$

We can rewrite this matrix if it is evaluated at an electroneutral configuration. Then, the salt concentration $c_{\text{salt}}$ is well defined such that

$$\boldsymbol{J}_{\tilde{\mu}} = \frac{n_+ + n_-}{n_+ n_-} \frac{d\mu_{\text{salt}}}{dc_{\text{salt}}} \begin{pmatrix} \gamma \left(1 + \frac{\rho_+}{\rho_{\text{N}}}\right) \frac{n_-}{n_+} & (1-\gamma) \frac{\rho_+}{\rho_{\text{N}}} \\ \gamma \frac{\rho_-}{\rho_{\text{N}}} & (1-\gamma) \left(1 + \frac{\rho_-}{\rho_{\text{N}}}\right) \frac{n_+}{n_-} \end{pmatrix}. \tag{SI-54}$$

In this case, the determinant of this matrix becomes

$$\begin{aligned}\det \boldsymbol{J}_{\tilde{\mu}} &= \gamma\,(1-\gamma)\cdot\left(\frac{n_+ + n_-}{n_+ n_-}\right)^2\cdot\left(\frac{d\mu_\mathrm{salt}}{dc_\mathrm{salt}}\right)^2\frac{\rho}{\rho_\mathrm{N}}\\ &= \gamma\,(1-\gamma)\cdot\left(\frac{n_+ + n_-}{n_+ n_-}\right)^2\cdot\frac{d\mu_\mathrm{salt}}{dc_\mathrm{salt}}\frac{d\tilde{\mu}_\mathrm{salt}}{dc_\mathrm{salt}}.\end{aligned} \tag{SI-55}$$

### B. Salt Diffusion Coefficient

Equation (SI-18) is used to express the anion flux with the assumption of a neutral concentration distribution

$$\begin{aligned}\mathrm{N}_- &= -\tilde{\Gamma}_{--}\nabla\tilde{\tilde{\mu}}_- + \frac{t_-\mathcal{J}}{z_-F}\\ &= -\tilde{\Gamma}_{--}\frac{n_+ + n_-}{n_-}\nabla\tilde{\mu}_\mathrm{salt} + \frac{t_-\mathcal{J}}{z_-F}\\ &= -\tilde{\Gamma}_{--}\frac{n_+ + n_-}{n_-^2}\frac{d\tilde{\mu}_\mathrm{salt}}{dc_\mathrm{salt}}\nabla c_- + \frac{t_-\mathcal{J}}{z_-F}.\end{aligned} \tag{SI-56}$$

Comparison to the canonical flux expression reveals that the diffusion coefficient $D_\mathrm{salt}$ is equal to $\tilde{\Gamma}_{--}\frac{n_+ + n_-}{n_-^2}\frac{d\tilde{\mu}_\mathrm{salt}}{dc_\mathrm{salt}}$. Note that this parameter is only well defined for fluxes relative to the center-of-mass velocity. With the definition of the shifted mobility coefficient $\tilde{\Gamma}_{--}$ as well as eq. (SI-41) the shifted mobility coefficient can be rewritten

$$\begin{aligned}\tilde{\Gamma}_{--} &= \Gamma_{--} - \frac{t_-}{z_-}\frac{t_-}{z_-}\frac{\kappa}{F^2} = \frac{F^2}{\kappa}\left(\frac{\kappa}{F^2}\Gamma_{--} - (z_-\Gamma_{--} + z_+\Gamma_{+-})^2\right)\\ &= \frac{F^2}{\kappa}\left(\left(z_+^2\Gamma_{++} + 2z_+z_-\Gamma_{+-} + z_-^2\Gamma_{--}\right)\Gamma_{--} - (z_-\Gamma_{--} + z_+\Gamma_{+-})^2\right)\\ &= \frac{z_+^2F^2}{\kappa}\left(\Gamma_{++}\Gamma_{--} - \Gamma_{+-}^2\right) = \frac{z_+^2F^2}{\kappa}\det\boldsymbol{\Gamma}.\end{aligned} \tag{SI-57}$$

Then, the equation which links the salt diffusion coefficient and the mobility coefficients $\Gamma_{\alpha\beta}$ becomes

$$\begin{aligned}D_\mathrm{salt} &= \frac{z_+^2F^2}{\kappa}\frac{n_+ + n_-}{n_-^2}\frac{d\tilde{\mu}_\mathrm{salt}}{dc_\mathrm{salt}}\det\boldsymbol{\Gamma}\\ &= -\frac{z_+z_-F^2}{\kappa}\frac{n_+ + n_-}{n_+n_-}\frac{\rho}{\rho_\mathrm{N}}\frac{d\mu_\mathrm{salt}}{dc_\mathrm{salt}}\det\boldsymbol{\Gamma}.\end{aligned} \tag{SI-58}$$

Here, the second transformation is done to show that the final expression for $D_\text{salt}$ is symmetric in $n_\pm$ and $z_\pm$. With eqs. (SI-41) and (SI-58) there are three equations to couple $D_\text{salt}, \kappa$ and $t_+$ to the three mobility coefficients. Inverting these equations results in

$$\Gamma_{\alpha\beta} = D_\text{salt} \left| \frac{z_+ z_-}{z_\alpha z_\beta} \right| \frac{n_+ n_-}{n_+ + n_-} \frac{\rho_\text{N}}{\rho} \left( \frac{d\mu_\text{salt}}{dc_\text{salt}} \right)^{-1} + \frac{t_\alpha t_\beta \kappa}{z_\alpha z_\beta F^2}, \tag{SI-59a}$$

$$\tilde{\Gamma}_{\alpha\beta} = D_\text{salt} \left| \frac{z_+ z_-}{z_\alpha z_\beta} \right| \frac{n_+ n_-}{n_+ + n_-} \frac{\rho_\text{N}}{\rho} \left( \frac{d\mu_\text{salt}}{dc_\text{salt}} \right)^{-1}. \tag{SI-59b}$$

After calculating the the mobility matrix we can express the diffusion matrix $\boldsymbol{D} = \boldsymbol{\Gamma} \boldsymbol{J}_{\tilde{\mu}}$ with the Jacobi matrix given by eq. (SI-55) .

### C. Flux Expressions

Transcribing the flux expressions derived in section SI-1 to the binary electrolyte is straight forward. The binary electrolyte has $N = 3$ species which are assigned as $1 \rightarrow \text{N}$, $2 \rightarrow +$, and $3 \rightarrow -$. Then, eqs. (SI-18), (SI-22) and (SI-24a) become

$$\text{N}_\alpha = -\sum_{\beta=\pm} D_{\alpha\beta} \nabla c_\beta - \frac{t_\alpha \kappa}{\tilde{z}_\alpha F} \nabla \phi_\text{E}, \qquad \alpha = \pm \tag{SI-60a}$$

$$\text{N}_- = -\tilde{\Gamma}_{--} \nabla \tilde{\tilde{\mu}}_- + \frac{t_- \mathcal{J}}{z_- F}, \tag{SI-60b}$$

$$\mathcal{J} = -\frac{\kappa}{F} \frac{t_-}{z_-} \nabla \tilde{\tilde{\mu}}_- - \kappa \nabla \tilde{\varphi}, \tag{SI-60c}$$

where the effective electrochemical potential is defined as

$$\tilde{\varphi} = \phi_\text{E} + \frac{\tilde{\mu}_+}{z_+ F}. \tag{SI-61}$$

Next, eqs. (SI-60b) and (SI-60c) are rewritten with the assumption of electroneutrality, i.e. $z_+ c_+ + z_- c_- = 0$. The chemical potentials defined in section SI-3 A are used to express $\nabla \tilde{\tilde{\mu}}_-$.

This results in

$$\mathrm{N}_- = -D_{\mathrm{salt}} \nabla c_- + \frac{t_- \mathcal{J}}{z_- F}, \tag{SI-62a}$$

$$\mathcal{J} = \frac{\kappa}{F} \frac{t_-}{z_+} \underbrace{\frac{n_+ + n_-}{n_+ n_-}}_{\mathcal{N}} \frac{d\tilde{\mu}_{\mathrm{salt}}}{dc_{\mathrm{salt}}} \nabla c_- - \kappa \nabla \tilde{\varphi}. \tag{SI-62b}$$

### D. Linearisation

Applying the linearisation to the binary electrolyte is straight forward. The convection correction matrix reads

$$\boldsymbol{\mathcal{C}} = \begin{pmatrix} 1 - c_{+,0}\tilde{\nu}_+ & -c_{+,0}\tilde{\nu}_- \\ -c_{-,0}\tilde{\nu}_+ & 1 - c_{-,0}\tilde{\nu}_- \end{pmatrix}, \tag{SI-63}$$

so that the convection corrected transport coefficients become

$$D^*_{\mathrm{salt}} = \frac{\rho_0}{\tilde{\rho}_{\mathrm{N},0}} D_{\mathrm{salt}}, \tag{SI-64a}$$

$$\boldsymbol{D}^* = \boldsymbol{\mathcal{C}} \boldsymbol{D} \tag{SI-64b}$$

$$t^*_+ = (1 - c_{+,0}\tilde{\nu}_{+,0})\, t_+ + c_{-,0}\tilde{\nu}_{-,0} t_-, \tag{SI-64c}$$

$$t^*_- = c_{+,0}\tilde{\nu}_{+,0} t_+ + (1 - c_{-,0}\tilde{\nu}_{-,0})\, t_-. \tag{SI-64d}$$

To obtain the salt diffusion coefficient in the resting frame, we replace $\boldsymbol{\Gamma}$ with $\boldsymbol{\Gamma}^* = \boldsymbol{\mathcal{C}}\boldsymbol{\Gamma}$ in eq. (SI-58). Considering that $\det \boldsymbol{\mathcal{C}}\boldsymbol{\Gamma} = \det \boldsymbol{\mathcal{C}} \cdot \det \boldsymbol{\Gamma}$ then gives the result above we use eq. (SI-35). Note that the density of the complete solution $\rho$ is an easily measured quantity which is not true for $\tilde{\rho}_{\mathrm{N}}$. As described in section SI-2, this quantity does not equal the density of the pure solvent and must be calculated with $\nu_{\mathrm{N}}$, partial molar volume of the solvent. Note that the convection corrected transference numbers satisfy $t^*_+ + t^*_- = 1$.

The flux boundary condition is derived in section SI-1 B, see eq. (SI-10). Its linearised

form for the binary electrolyte reads

$$\mathrm{N}^{*}_{\alpha,\mathrm{lin}}\left(x_{\mathrm{I}}\right)=\mathrm{N}_{\alpha,\mathrm{lin}}+\frac{c_{\alpha,0}}{c_{+,0}}\frac{\rho_{+,0}}{\rho_{0}}\frac{j^{*}_{\mathrm{I}}}{z_{+}F}=\begin{cases}\frac{j^{*}_{\mathrm{I}}}{z_{+}F} & \alpha=+,\\ 0 & \alpha=-.\end{cases} \tag{SI-65}$$

The only difference is that concentrations and densities are replaced with the constant values which define the reference state ($c_{\alpha,0}$, and $\rho_{+,0}$).

## SI-4. IMPEDANCE: ELECTRONEUTRAL SYSTEM WITH SEI

We use eq. (30) to determine the three coefficients $C$, $\hat{C}^{+}$, and $\hat{C}^{-}$. This calculation is performed with analytical tools resulting in

$$C=\frac{\varepsilon}{\tau}\hat{k}e^{ikL'}\left(\left(e^{2i\hat{k}L'}+e^{2i\hat{k}L}\right)\left(t_{-}-\hat{t}_{-}\right)-2\hat{k}e^{i\hat{k}(L'+L)}\left(\hat{t}_{-}-\frac{\rho_{+}}{\rho}\right)\right), \tag{SI-66a}$$

$$\begin{aligned}\hat{C}^{+}=&e^{i\hat{k}L'}\left(e^{2ikL'}-1\right)\frac{\varepsilon}{\tau}\hat{k}\left(t_{-}-\hat{t}_{-}\right)\\&-e^{i\hat{k}L}\left(k-\frac{\varepsilon}{\tau}\hat{k}+e^{2i\hat{k}L}\left(k+\frac{\varepsilon}{\tau}\hat{k}\right)\right)\left(\hat{t}_{-}-\frac{\rho_{+}}{\rho}\right),\end{aligned} \tag{SI-66b}$$

$$\begin{aligned}\hat{C}^{-}=&e^{i\hat{k}L'+L}\Bigg(e^{i\hat{k}L}\left(e^{2ikL'}-1\right)\frac{\varepsilon}{\tau}\hat{k}\left(t_{-}-\hat{t}_{-}\right)\\&-2e^{i\left(k+\hat{k}\right)L'}\left(t_{-}-\frac{\rho_{+}}{\rho}\right)\left(k\cos kL'-i\frac{\varepsilon}{\tau}\hat{k}\sin kL'\right)\Bigg).\end{aligned} \tag{SI-66c}$$

## SI-5. APPENDIX: GENERAL IMPEDANCE

### A. Dispersion Relation

The relation between the “wave-numbers” $k_{\alpha}$ and the frequency $\omega=2\pi f$ is called dispersion relation. We now determine this relation by calculating the eigenvectors $\vec{\eta}_{\alpha}$ and eigenvalues $\lambda_{\alpha}$ of the matrix $\boldsymbol{\mathcal{A}}_{\omega}=\boldsymbol{D}^{*-1}\left(\boldsymbol{\mathcal{T}}+i\omega\boldsymbol{\mathcal{I}}\right)$. For the binary system, these matrices

read

$$\boldsymbol{D}^{*-1} = \frac{1}{\det \boldsymbol{D}^*} \begin{pmatrix} D^*_{++} & D^*_{+-} \\ D^*_{-+} & D^*_{--} \end{pmatrix}, \text{ and} \tag{SI-67a}$$

$$\boldsymbol{\mathcal{T}}^* + i\omega \boldsymbol{\mathcal{I}} = \frac{1}{\varepsilon_0 \varepsilon_{\mathrm{R}}} \begin{pmatrix} \kappa t^*_+ + i\omega\varepsilon_0\varepsilon_{\mathrm{R}} & -\kappa t^*_+ n_+/n_- \\ -\kappa t^*_- n_-/n_+ & \kappa t^*_- + i\omega\varepsilon_0\varepsilon_{\mathrm{R}} \end{pmatrix}, \tag{SI-67b}$$

where, $\det \boldsymbol{D}^* = D^*_{++}D^*_{--} - D^*_{+-}D^*_{-+}$. Determining $\vec{\eta}_\alpha$ and $\lambda_\alpha$ is a lengthy calculation which is performed with computational tools (Mathematica). We scale the eigenvectors of $\boldsymbol{\mathcal{A}}$ so that their second entry equals 1, i.e., $\vec{\eta}_\alpha = (\eta_\alpha, 1)^{\mathrm{T}}$. Both, the eigenvalues and the eigenvectors are large expressions. However, they satisfy the following relations

$$A_k = \lambda_1 \cdot \lambda_2 = \frac{i\omega\left(i\omega\varepsilon_0\varepsilon_{\mathrm{R}} + \kappa\right)}{\varepsilon_0\varepsilon_{\mathrm{R}} \det \boldsymbol{D}^*}, \tag{SI-68a}$$

$$\begin{aligned} B_k &= \lambda_1 + \lambda_2 \\ &= \frac{\left(D^*_{++} + D^*_{--}\right) i\omega\varepsilon_0\varepsilon_{\mathrm{R}} n_+ n_- + \kappa\left(D^*_{++}t^*_- n_+ n_- + D^*_{+-}t^*_- n_-^2 + D^*_{-+}t^*_+ n_+^2 + D^*_{--}t^*_+ n_+ n_-\right)}{\varepsilon_0\varepsilon_{\mathrm{R}} n_+ n_- \det \boldsymbol{D}^*} \\ &= \frac{\left(D^*_{++} + D^*_{--}\right) i\omega\varepsilon_0\varepsilon_{\mathrm{R}} + \kappa D^*_{\mathrm{salt}}}{\varepsilon_0\varepsilon_{\mathrm{R}} \det \boldsymbol{D}^*}, \end{aligned} \tag{SI-68b}$$

and

$$A_\eta = \eta_1 \cdot \eta_2 = -\frac{\left(i\omega\varepsilon_0\varepsilon_{\mathrm{R}} + \kappa t_-\right) D^*_{+-} n_+ n_- + \kappa t_+ D^*_{--} n_+^2}{\left(i\omega\varepsilon_0\varepsilon_{\mathrm{R}} + \kappa t_+\right) D^*_{-+} n_+ n_- + \kappa t_- D^*_{++} n_-^2}, \tag{SI-69a}$$

$$\begin{aligned} B_\eta &= \eta_1 + \eta_2 \\ &= \frac{\left(D^*_{++} - D^*_{--}\right) i\omega\varepsilon_0\varepsilon_{\mathrm{R}} n_+ n_- + \kappa\left(D^*_{++}t^*_- n_+ n_- - D^*_{+-}t^*_- n_-^2 + D^*_{-+}t^*_+ n_+^2 - D^*_{--}t^*_+ n_+ n_-\right)}{\left(i\omega\varepsilon_0\varepsilon_{\mathrm{R}} + \kappa t^*_+\right) D^*_{-+} n_+ n_- - \kappa D^*_{++} t^*_- n_-^2}. \end{aligned} \tag{SI-69b}$$

Using these quantities $k_{1,2}$ and $\eta_{1,2}$ can be expressed as such

$$k_{1,2} = \sqrt{-\frac{B_k}{2} \pm \sqrt{\frac{B_k^2}{4} - A_k}}, \tag{SI-70a}$$

$$\eta_{1,2} = \frac{B_\eta}{2} \pm \sqrt{\frac{B_\eta^2}{4} - A_\eta}. \tag{SI-70b}$$

These expressions are used to calculate $k_\alpha$ and $\eta_\alpha$. Note that they cannot be used to match the eigenvalues to their corresponding eigenvectors correctly because the sign of the square root cannot be assigned without ambiguity. This also applies to eq. (SI-70a) where the outer square-root only determines $k_\alpha$ with respect to the sign. Below, this sign is chosen such that $\operatorname{imag} k_\alpha$ is negative.

### B. Double-Layer Thickness and Interface Capacity

An essential result of the non-neutral model is the so called dispersion relation given by eq. (SI-70a). This expression describes two characteristic length scales of first order perturbations at a given frequency. We discuss these length scales in the low frequency or stationary limit in section 3.2.2. In this limit, one length scale diverges whereas the other one attains a constant value. It is given by

$$\begin{aligned}\lambda_{\mathrm{DL}} &= \lim_{\omega\to 0} i{k_1}^{-1} = i\sqrt{-B_k(\omega=0)^{-1}} = \sqrt{B_k(\omega=0)^{-1}} = \sqrt{\frac{\varepsilon_0\varepsilon_{\mathrm{R}}}{\kappa}\frac{\det \boldsymbol{D^*}}{D^*_{\mathrm{salt}}}} \\ &= \sqrt{-\frac{\varepsilon_0\varepsilon_{\mathrm{R}}RT}{z_+z_-F^2}\cdot\frac{\mathcal{N}\mathcal{F}_{\mathrm{salt}}}{c_{\mathrm{salt}}}\cdot\gamma\,(1-\gamma)}. \qquad \text{(SI-71)}\end{aligned}$$

In the last step, we use $\boldsymbol{D^*} = \boldsymbol{\mathcal{C}}\boldsymbol{\Gamma}\boldsymbol{J}_{\tilde{\mu}}$ and $D^*_{\mathrm{salt}} = \det\boldsymbol{\mathcal{C}}D_{\mathrm{salt}}$. Furthermore, we use eq. (SI-58) to relate $\det\boldsymbol{\Gamma}$ with $D_{\mathrm{salt}}$ as well as eq. (SI-55) to express the determinant of the Jacobi matrix. $\lambda_{\mathrm{DL}}$ characterizes the spatial extend of charged interface layers. Its dependence on $\gamma$ and the anion valence $z_-$ is illustrated in fig. SI-1 . It is a physical property that affects measurable quantities such as the double-layer capacity $C_{\mathrm{DL}}$. We find the charge stored within the diffuse layer by integrating the charge density. For the interface at $x = L$ we approximate this quantity with

$$Q_{\mathrm{DL}} = \lambda_{\mathrm{D}}F\left(\eta_{1,\mathrm{H}}z_+ + z_-\right)C^+_{\mathrm{H}}, \qquad \text{(SI-72)}$$

by considering $\lambda_{\mathrm{DL}} \ll L$. At the same time, the potential drop across the diffuse layer is well approximated by

$$\Phi_{\mathrm{DL}} = F\Pi_1 C^+_{\mathrm{H}} = F\frac{z_+\eta_1 + z_-}{\varepsilon_0\varepsilon_{\mathrm{R}}}\lambda^2_{\mathrm{DL}}C^+_{\mathrm{H}}, \qquad \text{(SI-73)}$$

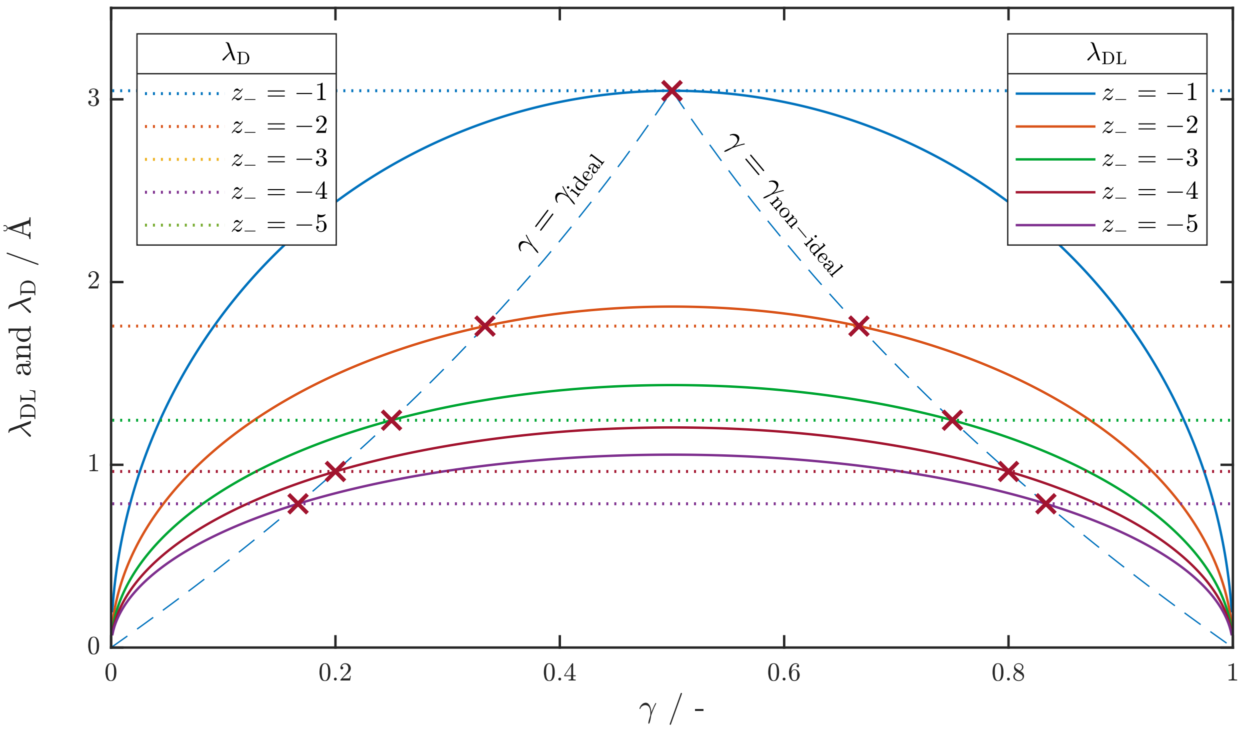


FIG. SI-1. Comparison between the double layer thickness $\lambda_{\mathrm{DL}}$ derived in this theory and the Debye length $\lambda_{\mathrm{D}}$. Both quantities have a similar parameter dependence, however, $\lambda_{\mathrm{DL}}$ additionally depends on $\gamma$, see eq. (SI-51a).

because $\lambda_{\mathrm{DL}} \ll {k_2}^{-1}$. Then, the interface capacity is equal to

$$C_{\mathrm{I}} = \frac{Q_{\mathrm{DL}}}{\Phi_{\mathrm{DL}}} = \frac{\varepsilon_0 \varepsilon_{\mathrm{R}}}{\lambda_{\mathrm{DL}}}. \qquad \text{(SI-74)}$$

This expression resembles the interface capacity given by the Debye theory, motivating a comparison between $\lambda_{\mathrm{DL}}$ and the Debye-screening length $\lambda_{\mathrm{D}}$. In a binary electrolyte, $\lambda_{\mathrm{D}}$ is given by

$$\lambda_{\mathrm{D}} = \sqrt{\frac{\varepsilon_0 \varepsilon_{\mathrm{R}} k_{\mathrm{B}} T}{N_{\mathrm{A}} e^2} \left(c_+ z_+^2 + c_- z_-^2\right)^{-1}} = \sqrt{\frac{\varepsilon_0 \varepsilon_{\mathrm{R}} R T}{F^2 c_{\mathrm{salt}}} \left(n_+ z_+^2 + n_- z_-^2\right)^{-1}}. \qquad \text{(SI-75)}$$

The factor $\sqrt{\varepsilon_0 \varepsilon_{\mathrm{R}} R T c_{\mathrm{salt}}^{-1} F^{-2}}$ scales both quantities equally. However, the expressions differ in the way they depend on the stoichiometry and valence of the salt. The exclusive appearance of $\mathcal{F}_{\mathrm{salt}}$ as well as $\gamma$ in eq. (SI-71) can be explained by the fact that the Debye theory is derived for a dilute and ideal solution of ions. This situation can be replicated in the theory derived here. Using ideal thermodynamic coefficients $\mathcal{F}_{\mathrm{salt}} = \mathcal{F}_+ = \mathcal{F}_- = 1$, see eq. (SI-51a),

results in an expression for $\gamma$

$$\gamma_{\text{ideal}} = \frac{n_+}{n_+ + n_-}. \tag{SI-76}$$

Both, $\lambda_{\text{DL}}$ and $\lambda_{\text{D}}$ align if this value is chosen for $\gamma$ and $\mathcal{F}_{\text{salt}}$ is equal to 1. This is also true if $\gamma = \gamma_{\text{non-ideal}} = \frac{n_-}{n_+ + n_-}$ although this no longer corresponds an ideal situation. This is illustrated in fig. SI-1.

To conclude, in terms of charged interface layers this theory aligns with the Debye-Hückel theory if ideal behaviour of all ionic species is assumed. This is surprising because the Debye-length is obtained by solving the (linearised) Poisson-Boltzmann equation. Therefore, the Boltzmann distribution is an essential part of the conventional derivation. In contrast, the derivation of $\lambda_{\text{DL}}$ is solely based on a set of thermodynamic consistent flux expressions, chemical potentials and the Poisson equation. The Boltzmann distribution is not used directly. However, an equivalent expression can be identified within the derivation. Note that $\lambda_{\text{DL}}$ is derived for in the stationary limit of a flux free reference state. This implies

$$\nabla \tilde{\mu}_\alpha^{\text{el}} = \nabla \left(\tilde{\mu}_\alpha + \tilde{z}_\alpha F \phi_{\text{E}}\right) = 0, \tag{SI-77}$$

if we consider the original flux expressions given by eq. (SI-11) Neglecting the solvent such that $\tilde{\mu}_\alpha = \mu_\alpha = \ln\left(f_\alpha c_\alpha c_{\alpha,0}^{-1}\right)$ then results in a link between the concentrations $c_\alpha$ and the potential $\phi_{\text{E}}$

$$\ln\left(f_\alpha c_\alpha\right) \propto -\frac{\tilde{z}_\alpha F \phi_{\text{E}}}{RT}, \qquad \text{or} \qquad f_\alpha c_\alpha \propto e^{-\frac{\tilde{z}_\alpha F \phi_{\text{E}}}{RT}}. \tag{SI-78}$$

The right hand side is equivalent to the Boltzmann distribution. In the Debye-Hückel theory, the exponential in this expression is linearised and the potential is expressed with the Poisson equation. This results in a second order differential equation where $\lambda_{\text{D}}$ emerges as a characteristic length. In this theory, linearisation is applied to the logarithm in the equivalent expression on the left hand side. Both theories use the Poisson equation to eliminate the electric field and are therefore equivalent for ideal systems.

### C. Non-Neutral System without SEI

The matrix equation eq. (64) defines the coefficient vector $\vec{C} = (C_1, C_2, \Phi')^{\mathrm{T}}$ with respect to its amplitude. The solution below is calculated with computational tools (Mathematica)

$$C_1 = -i\frac{\partial\mu_+}{\partial c_+}\eta_2 \sin k_2L\left(t_- - \frac{\rho_+}{\rho}\right) + \cos k_2LF^2\mathcal{R}z_+\left(t_+z_-\Omega_{-2} - t_-z_+\Omega_{+2}\right), \tag{SI-79a}$$

$$C_2 = F^2z_+\left(-i\Pi_1\sin k_1L\left(t_- - \frac{\rho_+}{\rho}\right) + \cos k_1L\mathcal{R}\left(t_-z_+\Omega_{+1} - t_+z_-\Omega_{-1}\right)\right), \tag{SI-79b}$$

$$\begin{aligned}\Phi' = &-2i\cos k_2LF^2\Pi_1\sin k_1Lz_+\left(z_-\Omega_{-2}\left(\frac{\rho_+}{\rho} - 1\right) + z_+\Omega_{+2}\frac{\rho_+}{\rho}\right)\\ &+ 2i\cos k_2LF^2\det\boldsymbol{\Omega}\mathcal{R}z_-z_+^2\\ &+ 2i\frac{\partial\mu_+}{\partial c_+}\eta_1\sin k_2L\left(z_-\Omega_{-1}\left(1 - \frac{\rho_+}{\rho}\right) - z_+\Omega_{+1}\frac{\rho_+}{\rho}\right).\end{aligned} \tag{SI-79c}$$

Note that the amplitude of the coefficient vector is not determined. However, this amplitude cancels out when calculating the impedance $Z$. We obtain the follwing expression when we calculate the impdance with eq. (1)

$$Z = \frac{\mathcal{A}}{\mathcal{B}}, \tag{SI-80}$$

where $\mathcal{A}$ and $\mathcal{B}$ are equal to

$$\begin{aligned}\mathcal{A} = L\Bigg(&\cos k_2LF^2\Pi_1\sin k_1Lz_+(\Omega_{-2}(-\rho + \rho_+)z_- + \Omega_{+2}\rho_+z_+)\\ &\quad + \cos k_1L(i\cos k_2LF^2(\Omega_{-1}\Omega_{+2} - \Omega_{-2}\Omega_{+1})\rho\mathcal{R}z_-z_+^2\\ &\qquad + \frac{\partial\mu_+}{\partial c_+}\eta_2\sin k_2L(\Omega_{-1}(-\rho + \rho_+)z_- + \Omega_{+1}\rho_+z_+))\Bigg)\\ &+ \kappa\Bigg(i\frac{\partial\mu_+}{\partial c_+}\eta_2\Pi_1\sin k_2L\sin k_1L(\rho t_- - \rho_+)\\ &\quad + F^2z_+\big(\cos k_2L\Pi_1\rho\mathcal{R}\sin k_1L(-\Omega_{-2}t_+z_- + \Omega_{+2}t_-z_+)\\ &\qquad + \Pi_2\sin k_2L(i\Pi_1\sin k_1L(\rho t_- - \rho_+) + \cos k_1L\rho\mathcal{R}(\Omega_{-1}t_+z_- - \Omega_{+1}t_-z_+))\big)\Bigg),\end{aligned} \tag{SI-81}$$

$$
\begin{aligned}
\mathcal{B} =& \varepsilon_0\varepsilon_\mathrm{R} i\omega \Bigg( \cos k_2 L F^2 \Pi_1 \sin k_1 L z_+ (\Omega_{-2}(-\rho+\rho_+)z_- + \Omega_{+2}\rho_+ z_+) \\
&+ \cos k_1 L (i \cos k_2 L F^2 (\Omega_{-1}\Omega_{+2} - \Omega_{-2}\Omega_{+1})\rho\mathcal{R} z_- z_+^2 \\
&+ \frac{\partial \mu_+}{\partial c_+}\eta_2 \sin k_2 L (\Omega_{-1}(-\rho+\rho_+)z_- + \Omega_{+1}\rho_+ z_+)) \Bigg) \\
&+ \kappa \Bigg[ \cos k_2 L F^2 \Pi_1 \sin k_1 L z_+ \big( i\varepsilon_0\varepsilon_\mathrm{R} i\omega k_2 \Pi_2 (\rho t_- - \rho_+) - \Omega_{-2}\rho t_+ z_- + \Omega_{+2}\rho t_- z_+ \big) \\
&+ \cos k_1 L \Bigg( \frac{\partial \mu_+}{\partial c_+}\eta_2 \sin k_2 L (i\varepsilon_0\varepsilon_\mathrm{R} i\omega k_1 \Pi_1 (\rho t_- - \rho_+) - \Omega_{-1}\rho t_+ z_- + \Omega_{+1}\rho t_- z_+) \\
&+ \cos k_2 L \varepsilon_0\varepsilon_\mathrm{R} F^2 i\omega\rho\mathcal{R} z_+ (k_1 \Pi_1 (-\Omega_{-2} t_+ z_- + \Omega_{+2} t_- z_+) + k_2 \Pi_2 (\Omega_{-1} t_+ z_- - \Omega_{+1} t_- z_+)) \Bigg) \Bigg].
\end{aligned}
\tag{SI-82}
$$

### D. Non-Neutral System with SEI

Below, we state the matrix $\boldsymbol{\mathcal{S}}$ for the non-neutral system with SEI. This is a 8x9 matrix where the first six lines correspond to the six continuity constraints at $x = L'$ listed in the main document. These equations are ordered from top to bottom $c_+$, $c_-$, $\Phi$, $\partial_x \Phi$, $\mathrm{N}_+$, and, $\mathrm{N}_-$. They are followed by the constraint for the flux boundary conditions for $\mathrm{N}_+$ and $\mathrm{N}_-$ at $x = L$.

$$
\boldsymbol{\mathcal{S}} = \begin{pmatrix}
-\eta_1 \sin k_1 L' & -\eta_2 \sin k_2 L' & 0 & \hat{\eta}_1 e^{ik_1 L'} & \hat{\eta}_1 e^{-ik_1 L'} & \hat{\eta}_2 e^{ik_2 L'} & \hat{\eta}_2 e^{-ik_2 L'} & 0 & 0 \\
-\sin k_1 L' & -\sin k_2 L' & 0 & 1 e^{ik_1 L'} & e^{-ik_1 L'} & e^{ik_2 L'} & e^{-ik_2 L'} & 0 & 0 \\
-\Pi_1 \sin k_1 L' & -\Pi_2 \sin k_2 L' & -L' & \hat{\Pi}_+ e^{ik_1 L'} & \hat{\Pi}_+ e^{-ik_1 L'} & \hat{\Pi}_- e^{ik_2 L'} & \hat{\Pi}_- e^{-ik_2 L'} & L & 1 \\
-\varepsilon_{\mathrm{R}} k_1 \Pi_1 \cos k_1 L' & -\varepsilon_{\mathrm{R}} k_2 \Pi_2 \cos k_2 L' & -\varepsilon_{\mathrm{R}} & i\hat{\varepsilon}_{\mathrm{R}} \hat{k}_1 \hat{\Pi}_+ e^{ik_1 L'} & -i\hat{\varepsilon}_{\mathrm{R}} \hat{k}_1 \hat{\Pi}_+ e^{-ik_1 L'} & i\hat{\varepsilon}_{\mathrm{R}} \hat{k}_2 \hat{\Pi}_- e^{ik_2 L'} & -i\hat{\varepsilon}_{\mathrm{R}} \hat{k}_2 \hat{\Pi}_- e^{-ik_2 L'} & \hat{\varepsilon}_{\mathrm{R}} & 0 \\
\Omega_{+1} \cos k_1 L' & \Omega_{+2} \cos k_2 L' & \frac{t_+ \kappa}{z_+ F} & -\hat{\Omega}_{+1} e^{ik_1 L'} & \hat{\Omega}_{+1} e^{-ik_1 L'} & -\hat{\Omega}_{+2} e^{ik_2 L'} & \hat{\Omega}_{+2} e^{-ik_2 L'} & -\frac{\hat{t}_+ \hat{\kappa}}{z_+ F} & 0 \\
\Omega_{-1} \cos k_1 L' & \Omega_{-2} \cos k_2 L' & \frac{t_- \kappa}{z_- F} & -\hat{\Omega}_{-1} e^{ik_1 L'} & \hat{\Omega}_{-1} e^{-ik_1 L'} & -\hat{\Omega}_{-2} e^{ik_2 L'} & \hat{\Omega}_{-2} e^{-ik_2 L'} & -\frac{\hat{t}_- \hat{\kappa}}{z_- F} & 0 \\
0 & 0 & 0 & -\hat{\Omega}_{+1} e^{ik_1 L} & \hat{\Omega}_{+1} e^{-ik_1 L} & -\hat{\Omega}_{+2} e^{ik_2 L} & \hat{\Omega}_{+2} e^{-ik_2 L} & -\frac{\hat{t}_+ \hat{\kappa}}{z_+ F} & 0 \\
0 & 0 & 0 & -\hat{\Omega}_{-1} e^{ik_1 L} & \hat{\Omega}_{-1} e^{-ik_1 L} & -\hat{\Omega}_{-2} e^{ik_2 L} & \hat{\Omega}_{-2} e^{-ik_2 L} & -\frac{\hat{t}_- \hat{\kappa}}{z_- F} & 0
\end{pmatrix}
$$

$$
+ \frac{1}{\tilde{\mathcal{R}}} \underbrace{\begin{pmatrix}
0 & \cdots & & \cdots & 0 \\
\vdots & \ddots & & & \vdots \\
 & & 0 & 0 & 0 \\
\vdots & & 0 & \frac{\rho_0 - \rho_{+,0}}{z_+ F \rho_0} & 0 \\
0 & \cdots & 0 & 0 & \frac{1}{z_- F} \frac{\rho_{+,0}}{\rho_0}
\end{pmatrix}}_{9 \times 8}
\begin{pmatrix}
0 & \cdots & & & & & & \cdots & 0 \\
\vdots & & & & & & & & \vdots \\
0 & \cdots & & & & & & \cdots & 0 \\
0 & 0 & 0 & F\hat{\Pi}_+ e^{ik_1 L} & F\hat{\Pi}_+ e^{-ik_1 L} & \frac{\hat{\eta}_2 \partial \mu_+}{z_+ F} e^{ik_2 L} & \frac{\hat{\eta}_2 \partial \mu_+}{z_+ F} e^{-ik_2 L} & 0 & 0 \\
0 & 0 & 0 & F\hat{\Pi}_+ e^{ik_1 L} & F\hat{\Pi}_+ e^{-ik_1 L} & \frac{\hat{\eta}_2 \partial \mu_+}{z_+ F} e^{ik_2 L} & \frac{\hat{\eta}_2 \partial \mu_+}{z_+ F} e^{-ik_2 L} & 0 & 0
\end{pmatrix}
\tag{SI-83}
$$

## SI-6. INTERCALATION ELECTRODES

In this section we briefly discuss the impedance response of an intercalation electrode. The electrode material has an equilibrium potential $U(c_{\mathrm{S}})$ which depends on the degree of lithiation, i.e., the solid concentration $c_{\mathrm{S}}$. We consider this in the linearised overpotential eq. (11). Here only the first order term is used to approximate the change of the electrode potential as the solid concentration at the electrode surface changes. We introduce

$$\partial U = \left.\frac{\partial U}{\partial c_{\mathrm{S}}}\right|_{cS=c_{\mathrm{S},0}} = \frac{1}{c_{\mathrm{S,max}}} \left.\frac{\partial U}{\partial \mathrm{SoC}}\right|_{\mathrm{SoC}=\mathrm{SoC}_0}, \tag{SI-84}$$

to express the linearised reaction rate as follows

$$j_{\mathrm{I}}\mathcal{R} = \underbrace{\delta\phi_{\mathrm{S}} - \delta\varphi^{\mathrm{bulk}}}_{\eta_{\mathrm{H}}} - \partial U \delta c_{\mathrm{S}}. \tag{SI-85}$$

Here, $\eta_{\mathrm{H}}$ contains all contributions to the overpotential that are considered in the main document.

We consider a planar electrode with thickness $L_{\mathrm{S}}$. A similar calculation is performed by Meyers et al.[5] for spherical electrode particles. We shift the coordinate system such that the interface reaction takes place at $x = L_{\mathrm{S}}$ and the electrode begins at $x = 0$. It is assumed that the electronic conductivity of these particles is large such that all potential gradients in the particles are zero. The absence of electric potential gradients also implies that diffusion is the only relevant transport process for the solid species. We therefore use the linearised flux expression to describe transport of the intercalated species

$$N_{\mathrm{S,lin}} = -D_{\mathrm{S},0} \nabla \delta c_{\mathrm{S}}. \tag{SI-86}$$

Here, $D_{\mathrm{S},0}$ is the solid diffusion coefficient at the reference concentration $c_{\mathrm{S},0}$. Using this expression in a mass-balance equation results in an ODE for $c_{\mathrm{S}}$

$$\partial_t \delta c_{\mathrm{S}} = D_{\mathrm{S}} \boldsymbol{\Delta} c_{\mathrm{S}} = D_{\mathrm{S}} \frac{\partial \delta c_{\mathrm{S}}}{\partial x}. \tag{SI-87}$$

Again, we solve this equation is solved with an exponential ansatz

$$\delta c_{\mathrm{S}} = e^{i\omega t} e^{iqx}. \tag{SI-88}$$

Inserting the ansatz in eq. (SI-87) results in the dispersion relation

$$q = \pm (1 - i) \sqrt{\frac{\omega}{2D_{\mathrm{S}}}}. \tag{SI-89}$$

The solution of $\delta c_{\mathrm{S}}$ is given by a linear combination of eq. (SI-88) with both solutions $\pm q$. This linear combination must satisfy flux boundary conditions at $x = 0$ and $x = L_{\mathrm{S}}$. At $x = 0$, the flux in the electrode must be zero because of the adjacent current collector. This eliminates one coefficient and implies

$$\delta c_{\mathrm{S}} = e^{i\omega t} \cdot C_{\mathrm{S}} \cos(qx), \tag{SI-90}$$

where $C_{\mathrm{S}}$ is the remaining coefficient of the linear combination. This is the time dependent solution of the lithium concentration in the electrode for the frequency $\omega$. Using this solution to express the flux at $x = L_{\mathrm{S}}$ results in

$$\mathrm{N}_{\mathrm{S}}(L_{\mathrm{S}}) = e^{i\omega t} \cdot C_{\mathrm{S}} D_{\mathrm{S},0} q \sin(qL_{\mathrm{S}}). \tag{SI-91}$$

This expression must equal the rate of the interface reaction given by eq. (SI-85) such that

$$C_{\mathrm{S}} = \frac{\eta_{\mathrm{H}}}{e^{i\omega t}} \left( \partial U \cos\left(qL_{\mathrm{S}}\right) + z_{+} F \mathcal{R} D_{\mathrm{S},0} \sin(qL_{\mathrm{S}}) \right)^{-1}. \tag{SI-92}$$

This is then used with eq. (SI-91) to find the reaction rate $j_{\mathrm{I}}$

$$j_{\mathrm{I}} = z_{+} F \mathrm{N}_{\mathrm{S}}(L_{\mathrm{S}}) = \frac{\eta_{\mathrm{H}}}{\mathcal{R} + \frac{\partial U}{z_{+} F q D_{\mathrm{S},0}} \tan(qL_{\mathrm{S}})^{-1}} = \frac{\eta_{\mathrm{H}}}{\tilde{\mathcal{R}}}. \tag{SI-93}$$

All contributions from the oscillating concentration at the electrode surface can be included

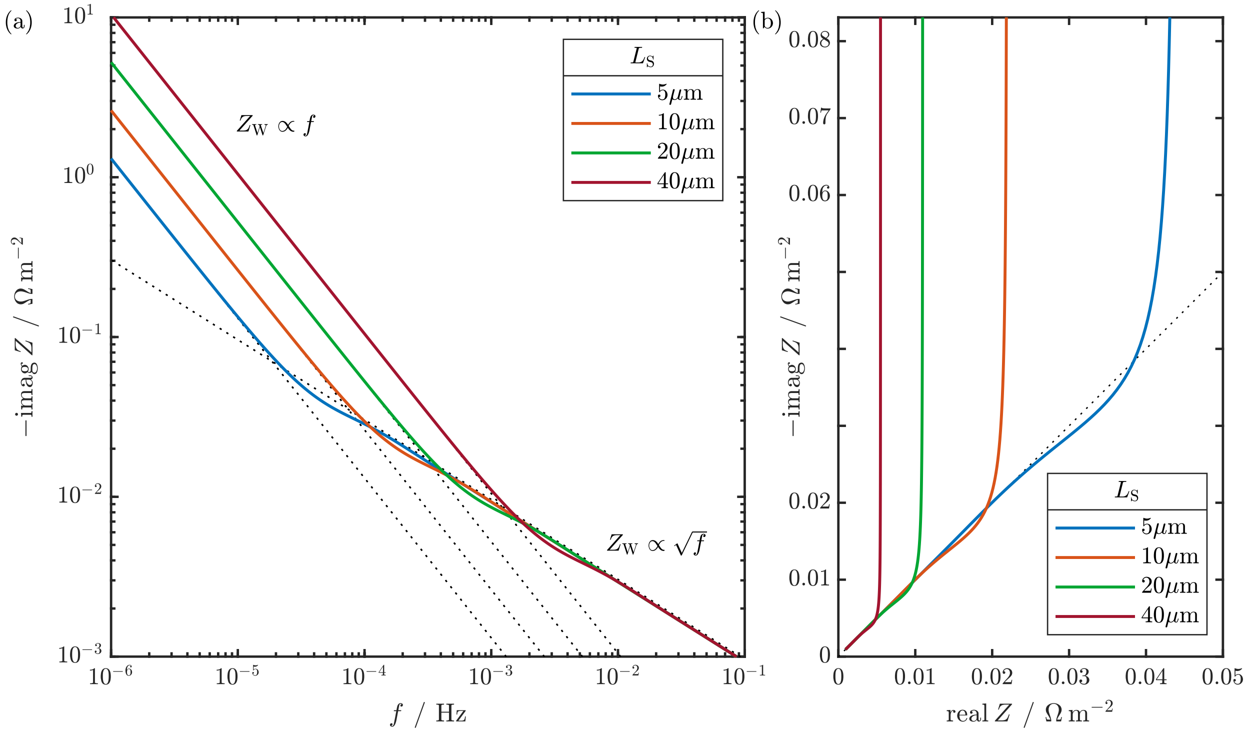


FIG. SI-2. The Warburg impedance of a graphite layer of varying thickness. (a) Bode Plot and (b) complex impedance. Parameters used: $c_{\mathrm{S,max}} = 31507\,\mathrm{mol\,m^{-3}}$, $\frac{\partial U}{\partial \mathrm{SoC}} = -1\,\mathrm{V}$, $D_\mathrm{S} = 10^{-13}\,\mathrm{m^2/s}$.

in the effective interface resistance $\tilde{\mathcal{R}}$

$$\tilde{\mathcal{R}} = \mathcal{R} + \underbrace{\frac{\partial U}{z_+ F q D_{\mathrm{S},0}} \tan\left(q L_\mathrm{S}\right)^{-1}}_{Z_\mathrm{W}} . \tag{SI-94}$$

This resistance depends on the frequency via $q$ which is given by eq. (SI-89). $Z_\mathrm{W}$ is the so-called Warburg impedance that increases the interface resistance at low frequencies. We depict it in fig. SI-2. Note that this effect vanishes if $\partial U$ is zero. Consequently, this Warburg resistance is only encountered for intercalation electrodes.

## SI-7. LIST OF PARAMETERS

TABLE SI-1: Parameters used for figures in this section.

(1) $n_+\nu_+ + n_-\nu_-$ is calculated with the experimentally obtained value of the density of the salt solution $\rho_0$ and the value for $\nu_N$. $\nu_+$ is assumed.

(2) Because of a lack of experimental data we use the molar volumes of pure solvent for the partial molar volumes of the solvent.

| | Unit | $LiPF_6$ EC/DMC (1:1 wt.-%) | LiTFSI Tetraglyme | Comment |
|---|---|---|---|---|
| $z_{+/-/N}$ | - | $1/-1/0$ | $1/-1/0$ | |
| $n_{+/-}$ | - | 1/1 | 1/1 | |
| $M_+$ | $g\,mol^{-1}$ | 6.94 | 6.94 | |
| $M_-$ | $g\,mol^{-1}$ | 144.96 | 287.09 | |
| $M_N$ | $g\,mol^{-1}$ | 88.06/90.08 (89.08*) | 222.28 | Weighted average |
| $\nu_+$ | $cm^3\,mol^{-1}$ | 20.0 | 20.0 | See caption (1) |
| $\nu_-$ | $cm^3\,mol^{-1}$ | 106.8 | 122.75[6] | See caption (1) |
| $\nu_N$ | $cm^3\,mol^{-1}$ | 75.93[7] | 220.89[6] | See caption (2) |
| $c_{salt,0}$ | $mol\,l^{-1}$ | 1.0 | 2.75 | |
| $c_{N,0}$ | $mol\,l^{-1}$ | 13.17 | 2.75[8] | Calculated with eq 29 in[8] |
| $D^*_{salt}$ | $m^2\,s^{-1}$ | $1.5 \cdot 10^{-10*}$ | $8.9 \cdot 10^{-12*}$ | Calculated with data from[8] |
| $\kappa$ | $S\,m^{-1}$ | 1.16[8] | 0.152[8] | |
| $t_+$ | $mol\,l^{-1}$ | 0.063*[8] | 0.025*[8] | |
| $\mathcal{F}_{salt}$ | - | 3.47* | 6.2* | Calculated with data from[8] |
| $\gamma$ | - | 0.5 | 0.5 | Equal to $\gamma_{ideal}$ |
| $\varepsilon_R$ | - | 31.41*[7] | 7.71[6] | See caption (3) |

TABLE SI-2: Parameters used for impedance fit to the experimental data from Wohde et al.[8] discussed in section 5 and shown in fig. 8.

| | Unit | Parameter Set | | Comment |
|---|---|---|---|---|
| | | I | II | |
| $\mathcal{R}$ | $\Omega\,cm^2$ | 95 | 13 | |
| $\zeta$ | - | 5 | 0.02 | |
| $\hat{t}_+$ | - | 0.90 | 0.97 | |
| $\hat{\varepsilon}_R$ | - | 131 | 347 | |
| $\varepsilon$ | - | 0.1 | | |
| $\tau$ | - | 3450 | | |
| $\hat{L}$ | nm | 25 | 67 | |
| $A$ | $cm^2$ | 1.131 | | Obtained from the authors of[8] |


[*] Corresponding author: birger.horstmann@dlr.de

[†] Corresponding author: arnulf.latz@dlr.de



[1] M. Schammer, A. Latz, and B. Horstmann, In Submission (2019).

[2] A. Latz and J. Zausch, Journal of Power Sources **196**, 3296 (2011).

[3] J. Stamm, A. Varzi, A. Latz, and B. Horstmann, Journal of Power Sources **360**, 136 (2017), arXiv:1612.03464.

[4] S. Clark, A. Latz, and B. Horstmann, ChemSusChem **10**, 4735 (2017).

[5] J. P. Meyers, M. Doyle, R. M. Darling, and J. Newman, Journal of The Electrochemical Society **147**, 2930 (2000).

[6] D. Brouillette, G. Perron, and J. E. Desnoyers, Journal of Solution Chemistry **27**, 151 (1998).

[7] R. Naejus and D. Lemordant, The Journal of Chemical Thermodynamics **29**, 1503 (1997).

[8] F. Wohde, M. Balabajew, and B. Roling, Journal of The Electrochemical Society **163**, A714 (2016).
